# Supplementary material for: Constrained Reinforcement Learning with Smoothed Log Barrier Function
Source: arXiv:2403.14508 source file (2024-03-21)
Supplement: Supplementary file 1 [file appendix.tex]

\section{Appendix}
In the Appendix, we provide the hyperparameters that we use to conduct our experiments. We also provide more details about the training environments and additional experiment results.
\subsection{Hyperparameters}
\label{sec:hyperparameters}
We use Adam Optimizer~\cite{DBLP:journals/corr/KingmaB14}.
Our implementations for CSAC-LB, SAC-Lag, WCSAC and SAC with Reward shaping are based on stable-baselines3~\citep{DBLP:journals/jmlr/RaffinHGKED21}.
The hyperparameters we used for all environments except SafetyPointGoal1 are the default hyperparameters used in stable-baselines3.
We summarize the common hyperparameters in Table~\ref{tab:common_hp}. The specific hyperparameters of the different algorithms are included in Tables~\ref{tab:sac_hp}, \ref{tab:csac_hp}, \ref{tab:sac_lag_hp}, \ref{tab:wcsac_hp} and \ref{tab:recoveryrl_hp}. The changes of hyperparameters in SafetyPointGoal1 are summarized in~Tab.~\ref{tab:new_hp_pointgoal1}.

\subsection{Neural Architecture}
For SAC with reward shaping, WCSAC, SAC-Lag and CSAC-LB, we use two layers of Multilayer Perceptron with 256 units per layer for all environments other than SafetyPointGoal1 and ReLU activation function as the reward/cost critic and actor network. The logarithmic standard deviation of the Gaussian output distribution of the actor network is clipped to $(-20, 2)$. In SafetyPointGoal1 Environment, we uses 512 units per layer and the rest stays the same.

For Recovery RL, we use the same actor critic architectures for fair comparison. The risk critic has the same architecture as the return critic except that a Sigmoid activation at the output. 
    
\subsection{Proof of Performance Guarantee Bound}

\begin{proof} 
We use $\mathit{J}(\pi_{\phi})$ to refer the objective of SAC as defined in Eq.~\ref{eq:sac_ori_objective} and $g(\pi_{\phi})$ now refers to the cost function of the constraint violations as the second line of Eq.~\ref{eq:rl_cons_prob}. We convert the maximization problem to minimization problem by negating the $\mathit{J}(\pi_{\phi})$. Then we obtain:
\begin{gather}
\label{eq:rl_cons_prob_append}
\min_{\phi} -\mathit{J}(\pi_{\phi}) \\
\textrm{s.t.} ~ g_{i}(\pi_{\phi}) \leq 0 ~~~ \forall{i \in {\{1, ..., m\}}} \nonumber
\end{gather}

The Lagrangian function of \ref{eq:rl_cons_prob_append} can then be written as:
\begin{align}
\label{eq:lag_appendix}
\mathit{L} (x, \lambda) = - \mathit{J}(\pi_{\phi}) + \sum_{i=1}^{m} \lambda_{i} g_{i}(\pi_{\phi})
\end{align}
where $\lambda_{i}$ is the Lagrangian multiplier and $\lambda_{i} \geq 0, ~~ \forall{i \in {\{1, ..., m\}}}$ 

The dual function is
\begin{align}
q(\lambda_{i}) = - \mathit{J}(\pi_{\phi})) + \sum_{i=1}^{m} \lambda_{i}g_{i}(\pi_{\phi})
\end{align}

We denote that the optimal solution of the unconstrained problem (Eq.~\ref{eq:csac_loss}) using the modified log barrier function is $\phi^{*}$. Therefore, the optimal parametrized policy can be written as $\pi_{\phi^{*}}$.

If the unconstrained problem is feasible, the optimal solution $\phi^{*}$ satisfies
\begin{align}
- \nabla{\mathit{J}(\pi_{\phi^{*}})} + \sum_{i=1}^{m} \Tilde{\phi}'_{t}(g_i({\pi_{\phi^{*}}})) \nabla{g_{i}(\pi_{\phi^{*}})} = 0
\end{align}

where $g_{i}(\pi_{\phi^{*}}) \leq 0 ~~~ \forall{i \in {\{1, ..., m\}}}$

We define
\begin{align}
    \lambda^{*}_{i} = \Tilde{\phi}'_{t}(g_i({\pi_{\phi^{*}}}))
\end{align}
Then we can obtain
\begin{align}
- \nabla{\mathit{J}(\pi_{\phi^{*}})} + \sum_{i=1}^{m} \lambda^{*}_{i} \nabla{g_{i}(\pi_{\phi^{*}})} = 0
\end{align}
From this, we can see that $\phi^{*}$ minimizes the Lagrangian Equation as defined in Eq.~\ref{eq:lag_appendix} when $\lambda_{i} = \lambda^{*}_{i}$,

We define $p^{*}$ as the optimal value of the original problem~(Eq.\ref{eq:rl_cons_prob}). Then we have $p^{*} > q(\lambda^{*}_{i})$
Therefore, 
\begin{align}
- \mathit{J}(\pi_{\phi^{*}})) - p^{*} \leq -\sum_{i=1}^{m} \lambda^{*}_{i}g_{i}(\pi_{\phi^{*}})
\end{align}

Given that
\begin{align}
\label{eq:gradient_ext_log_barrier}
\Tilde{\phi}'(z) = \begin{cases}
      0 & \text{if $z \leq 0$} \\
      \frac{1}{(z-1)\mu} & \text{if $0 < z \leq 1-\frac{1}{\mu^2}$}\\
      \mu & \text{otherwise}
    \end{cases}       
\end{align}

Given $\mu$ is the logarithmic barrier function factor, which is a hyperparameter and $\mu > 0$, we now consider all three cases for each term in $-\sum_{i=1}^{m} \lambda^{*}_{i}g_{i}(\pi_{\phi^{*}})$
\begin{itemize}
  \item If $g_{i}(\pi_{\phi^{*}}) \leq 0$,~~ $-\lambda^{*}_{i}g_{i}(\pi_{\phi^{*}}) = 0$
  \item If $0 < g_{i}(\pi_{\phi^{*}}) \leq 1-\frac{1}{\mu^2}$,~~ $- \lambda^{*}_{i}g_{i}(\pi_{\phi^{*}}) \leq \frac{\mu^{2}-1}{\mu}$
  \item  If $0 < g_{i}(\pi_{\phi^{*}}) > 1-\frac{1}{\mu^2},~~ - \lambda^{*}_{i}g_{i}(\pi_{\phi^{*}}) \leq \frac{1-\mu^{2}}{\mu}$
\end{itemize}
In all three cases, $-\lambda^{*}_{i}g_{i}(\pi_{\phi^{*}}) \leq \frac{|1-\mu^{2}|}{\mu}$. Therefore, we can conclude that
\begin{align}
- \mathit{J}(\pi_{\phi^{*}})) - p^{*} \leq -\sum_{i=1}^{m} \lambda^{*}_{i}g_{i}(\pi_{\phi^{*}}) \leq \frac{|1-\mu^2|\cdot m}{\mu}
\label{eq:convergence_conclusion}
\end{align}
\end{proof}

This theoretical analysis shows that our method can obtain the optimal solution as the original problem when $\mu = 1$ and the problem is feasible. However, due to the usage of gradient descent and neural networks (non-convex problem), there is no guarantee to always learn a global optimum.
\begin{figure}[h]
    \centering
    \includegraphics[width=0.7\columnwidth]{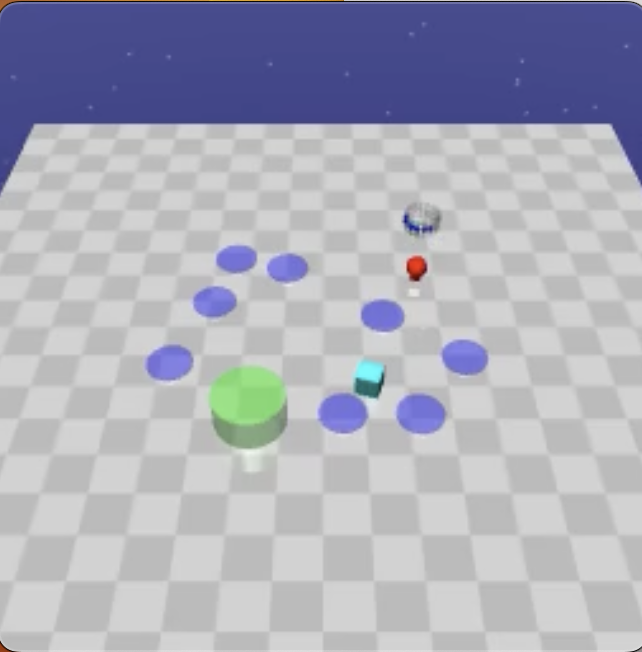}
    \caption{SafetyPointGoal1 Environment. The agent needs to control the red robot to reach the green area and avoid collision with blue obstacles.}
    \label{fig:pointgoal}
\end{figure}

\subsection{Experimental Details}
Here we summarize the setup of all four risk-sensitive tasks.

(a) \textbf{Tilt}: This is a modified version of Pendulum-v0 in OpenAI Gym~\citep{DBLP:journals/corr/BrockmanCPSSTZ16}. The reward function $r(s,a) = -\theta^{2}$, where $ \theta$ is the angle (in radian) between the pole and the vertical line. The constraint is $| \theta | \leq 1.5$, which is almost equivalent to $90^{\circ}$.  The horizon is 200.

(b) \textbf{Upright}: The constraint and horizon are the same as Tilt, but the reward function is $r(s,a) = - (\theta_{lim} - \theta)^{2}$, where $\theta_{lim} = -0.41151684$, which is the largest angle that a pole can stay balanced.

(c) \textbf{Move}: This is a modified version of the control task InvertedPendulum-v0 in Mujoco from OpenAI Gym. The reward function is $r(s,a) = x^2$, where $x$ is the position of cart. $\theta$ is the angle (in radian) between pole and the vertical line. The constraints are $| \theta | \leq 0.2$, which is close to $11^{\circ}$ and $| x | \leq 0.9$. The horizon is 1000.

(d) \textbf{Swing}: The environment and horizon are the same as Move. But the reward function is $r(s,a) = \theta^{2}$ and the constraints are $| \theta | \leq 1.5$ and $| x | \leq 0.9$.

The observation space of Tilt and Upright tasks has 3 dimensions, which are $cos(\theta)$, $sin(\theta)$ and the angular velocity. $\theta$ is the angle between the pole and the vertical line. The action space has only one dimension, which is the torque applied to pendulum.

Move and Swing tasks have 4 dimensions, which are the position of the cart along the horizon surface, vertical angle of the pole, velocity of the cart and the angular velocity of the pole. The action space also has 1 dimension, which is the force applied on the cart.

In the heating system environment, the observation space consists of the room temperature, return water temperature, wall temperature, ambient temperature, solar radiation, and energy from human activity, in total 6 dimensions. The action space has 1 dimension, which is the desired temperature of the room. The RL agent does not access to the low-level control of the heat pump, i.e. the power of the heat pump.

In the SafetyPointGoal1 Environment as depicted in Fig.~\ref{fig:pointgoal}, the observation space has 60 dimensions consisting of the data read from lidar sensor, accelerometer, velocimeter, gyro and magnetometer. The action space has two dimensions controlling the speed up/down or left/right directions. Cost is set to 1 when the robot collides with obstacles. The horizon is 1000.

\begin{figure}[h]
    \centering
    \includegraphics[width=0.9\columnwidth]{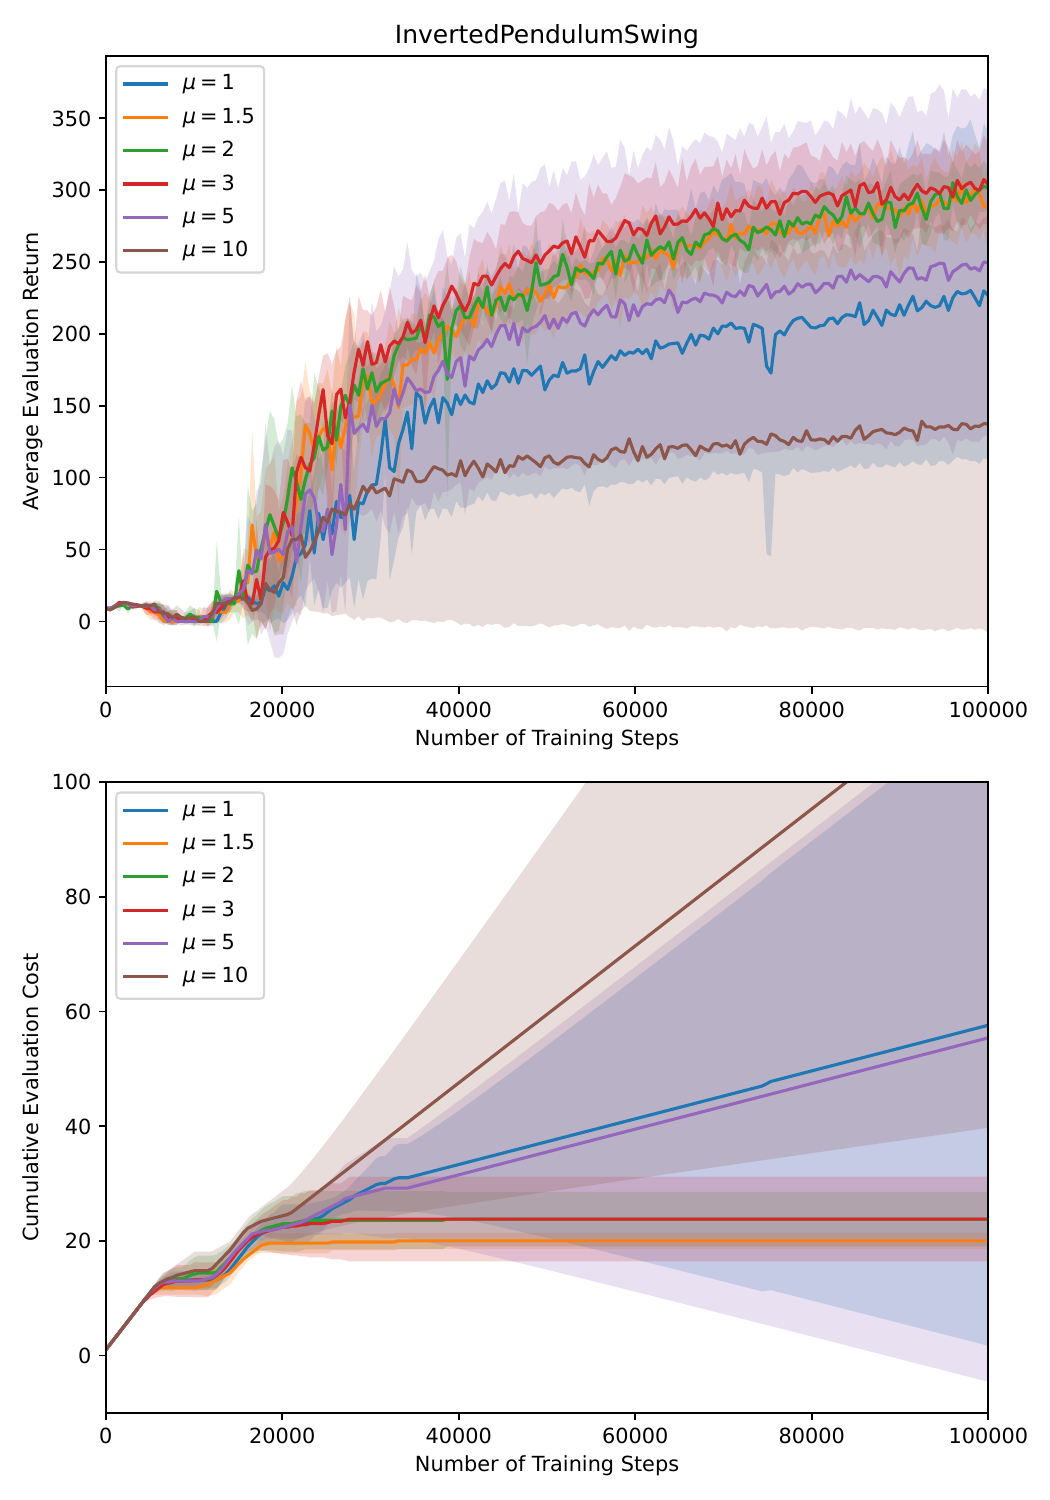}
    \caption{With the same setup as in Fig.~\ref{fig:safe_res}, we run 5 seeds for different log barrier factors $\mu$ in the Swing task. When $\mu$ is in a reasonable range, the performance is very similar.}
    \label{fig:ablation}
\end{figure}

\subsection{Ablation Study} 
To see the effect of different log barrier factors, we perform an ablation study in the Swing task. Fig.~\ref{fig:ablation} shows the effect of the log barrier factor on return and cost. When the log barrier factor is too large, due to the large gradient, the optimization is unstable and can thus cause an unstable policy. When the log barrier factor is set to 1, which results in a very small penalty on constraint violations and loses the property of a continuously smooth gradient when constraints are violated, the agent can not learn a proper policy. However, if we select a log barrier function between $1.5$ to $3$, the performance is very robust. This property ensures that CSAC-LB does not need to be tuned extensively to get a stable policy.

\begin{figure}[h]
    \centering
    \includegraphics[width=0.9\columnwidth]{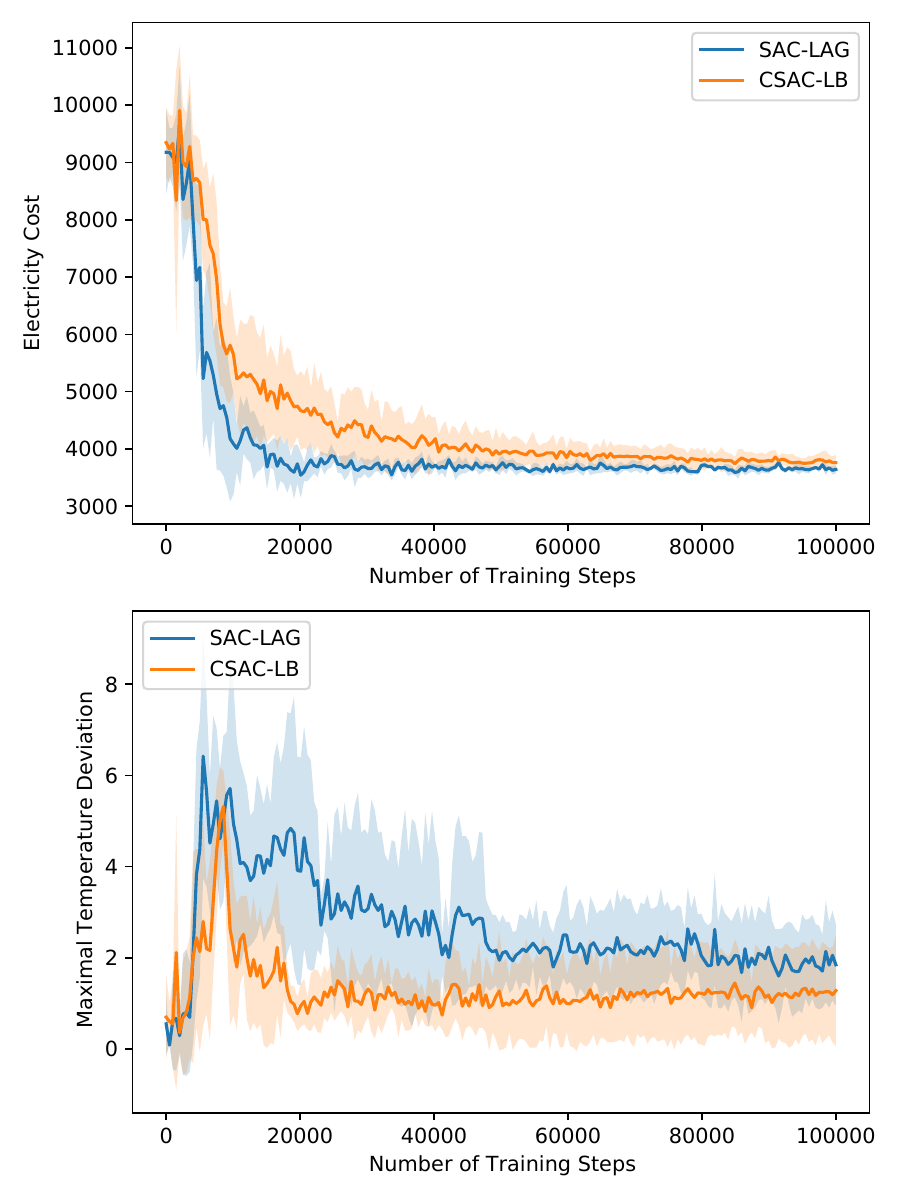}
    \caption{\textbf{Upper}: the average evaluation electricity cost in kWh over a year. \textbf{Lower}: the average maximal temperature deviation in Celsius over a year. The $x$-axis is the number of training steps. The faint area is the standard deviation. We run 5 seeds for each algorithm and every evaluation is carried out every 9600 steps~(equivalent to evaluate every 10 days of simulation.}
    \label{fig:heat_curves}
\end{figure}

\subsection{Additional Result}
We also evaluate SAC-Lag and CSAC-LB with 5 seeds each. Our result in Fig.~\ref{fig:heat_curves} again shows that CSAC-LB is able to perform better than SAC-Lag in the risk-neutral task. CSAC-LB is able to quickly decrease the maximal temperature deviation and decrease the electricity cost at the same time, whereas SAC-Lag is able to decrease the electricity cost but have relatively large constraint violations. In the end of the training, CSAC-LB is able to use similar energy to achieve less constraint violations. This result also matches the analysis we have in Fig~\ref{fig:heat_comp}.

    % ------------------------
    % Table for hyperparameters
    \begin{table*}[h]
    	\caption{The common hyperparameters of CSAC-LB, SAC-Lag, WCSAC and SAC with Reward shaping}
    	\begin{center}
    	\begin{small}
    		\begin{sc}
    		  \scalebox{0.8}{
			\begin{tabular}{lcll}
				\toprule
				\textbf{Hyperparameters} & \textbf{Value} & \textbf{Description}  \\
				\midrule
			batch size & 256 & The number of transitions for each update \\
			discount factor $\gamma$ & 0.99 & The importance of future rewards  \\
			replay buffer size & 1e6 & The maximum number of transitions stored in memory \\
			max training step & 1e6 & The number of training steps \\
			random steps & 100 & The number of randomly acting steps at the beginning \\
% 			total training steps & 100000 & The number of training steps \\
			actor learning rate & 3e-4 & The learning rate for actor network \\
			actor update frequency & 1 & The frequency for updating actor network \\
			critic learning rate & 3e-4 & The learning rate for critic network \\ 
			critic target update frequency & 2 & The frequency for updating critic target network \\
			polyak update factor & 0.005 & The update coefficient of critic target network for soft learning \\
			init temperature & 1.0 & initial temperature of actor's output for exploration \\
			temperature learning rate & 3e-4 & The learning rate for updating the policy entropy \\
			normalize observation & True & Normalize the observation by subtracting the mean and dividing the std\\
			normalize action & True & Normalize the action to $(-1, 1)$\\
			normalize return & True & Normalize the return by dividing the std of the episodic return\\
			normalize cost & True & Normalize the cost by dividing the std of the episodic cost \\
			clip reward & (-10, 10) & Clip the reward to the defined range \\
			clip cost & (-10, 10) & Clip the reward to the defined cost \\
			cost limit & 0 & The limit of the cost \\
				\bottomrule 
			\end{tabular}
			}
    			\end{sc}
    		\end{small}
    	\end{center}
    	\label{tab:common_hp}
    \end{table*}

\begin{table*}[h]
	\caption{The specific hyperparameters of SAC with Reward Shaping}
	\begin{center}
	\begin{small}
		\begin{sc}
		  \scalebox{0.8}{
		\begin{tabular}{lcll}
			\toprule
			\textbf{Hyperparameters} & \textbf{Value} & \textbf{Description}  \\
			\midrule
		penalty of constraint violation & -30 &  Agent receives -30 as reward if constraints are violated  \\
			\bottomrule 
		\end{tabular}
		}
			\end{sc}
		\end{small}
	\end{center}
	\label{tab:sac_hp}
\end{table*}

\begin{table*}[h]
	\caption{The specific hyperparameters of CSAC-LB}
	\begin{center}
	\begin{small}
		\begin{sc}
		  \scalebox{0.8}{
		\begin{tabular}{lcll}
			\toprule
			\textbf{Hyperparameters} & \textbf{Value} & \textbf{Description}  \\
			\midrule
		log barrier factor & 3 & The log barrier factor $\mu$ in Eq.\ref{eq:ext_log_barrier} \\
			\bottomrule 
		\end{tabular}
		}
			\end{sc}
		\end{small}
	\end{center}
	\label{tab:csac_hp}
\end{table*}

\begin{table*}[h]
	\caption{The specific hyperparameters of SAC-Lag}
	\begin{center}
	\begin{small}
		\begin{sc}
		  \scalebox{0.8}{
		\begin{tabular}{lcll}
			\toprule
			\textbf{Hyperparameters} & \textbf{Value} & \textbf{Description}  \\
			\midrule
		initial lagrangian-multiplier value & 0 & The value of $\beta$ defined in Eq.\ref{eq:lag_eq} \\
		Lagrangian-multiplier learning rate & $ 3e-4 $ & The learning rate for updating $\beta$ \\
			\bottomrule 
		\end{tabular}
		}
			\end{sc}
		\end{small}
	\end{center}
	\label{tab:sac_lag_hp}
\end{table*}

\begin{table*}[h]
	\caption{The specific hyperparameters of WCSAC}
	\begin{center}
	\begin{small}
		\begin{sc}
		  \scalebox{0.8}{
		\begin{tabular}{lcll}
			\toprule
			\textbf{Hyperparameters} & \textbf{Value} & \textbf{Description}  \\
			\midrule
		initial lagrangian-multiplier value & 0 & The value of $\beta$ defined in Eq.\ref{eq:lag_eq} \\
		Lagrangian-multiplier learning rate & $ 3e-4 $ & The learning rate for updating $\beta$ \\
		risk level & 0.5 & The risk level defined in WCSAC~\citep{DBLP:conf/aaai/YangSTS21} \\
		damp scale & 10 & The factor to control the change speed of $\beta$ \\
			\bottomrule 
		\end{tabular}
		}
			\end{sc}
		\end{small}
	\end{center}
	\label{tab:wcsac_hp}
\end{table*}

\begin{table*}[h]
	\caption{The specific hyperparameters of Recovery RL}
	\begin{center}
	\begin{small}
		\begin{sc}
		  \scalebox{0.8}{
		\begin{tabular}{lcll}
			\toprule
			\textbf{Hyperparameters} & \textbf{Value} & \textbf{Description}  \\
			\midrule
		$\gamma_{risk}$ & 0.6 & the discount factor for constraints \\
		$\epsilon{risk}$ & $ 0.5 $ & The threshold of risk critic \\
		pos fraction & 0.3 & The fraction of positive examples for critic training \\
			\bottomrule 
		\end{tabular}
		}
			\end{sc}
		\end{small}
	\end{center}
	\label{tab:recoveryrl_hp}
\end{table*}

\begin{table*}[h]
	\caption{The hyperparameters changes in SafetyPointGoal1}
	\begin{center}
	\begin{small}
		\begin{sc}
		  \scalebox{0.8}{
		\begin{tabular}{lcll}
			\toprule
			\textbf{Hyperparameters} & \textbf{Value} & \textbf{Description}  \\
			\midrule
		$\gamma_{risk}$ & 0.999 & the discount factor for constraints in SAC-Lag, WCSAC and CSAC-LB \\
		max training step & 3e6 & The number of training steps \\
		actor learning rate & 1e-4 & The learning rate for actor network for all methods\\
		critic learning rate & 1e-4 & The learning rate for critic network for all methods\\
		log barrier factor & 18 & The log barrier factor $\mu$ in Eq.\ref{eq:ext_log_barrier} \\
			\bottomrule 
		\end{tabular}
		}
			\end{sc}
		\end{small}
	\end{center}
	\label{tab:new_hp_pointgoal1}
\end{table*}
